# Supplementary material for: MultiDiff: Consistent Novel View Synthesis from a Single Image
Source: arXiv:2406.18524 source file (2024-06-26)

TSED scores on RealEstate10K at 128px resolution

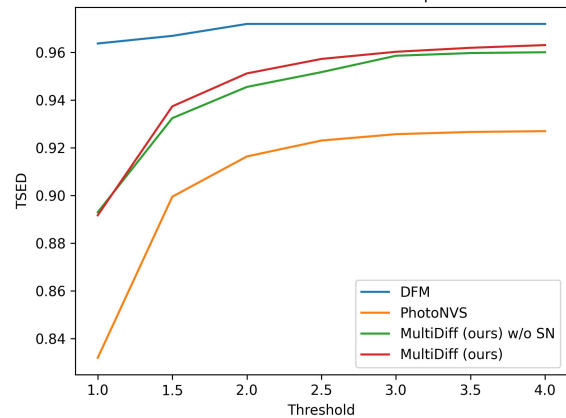

TSED@2px on RealEstate10K at 128px resolution

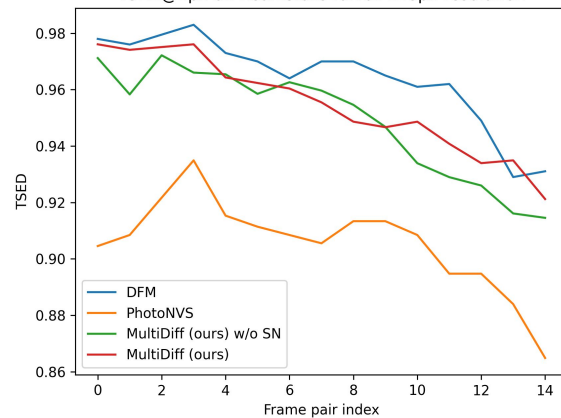

TSED scores on ScanNet at 128px resolution

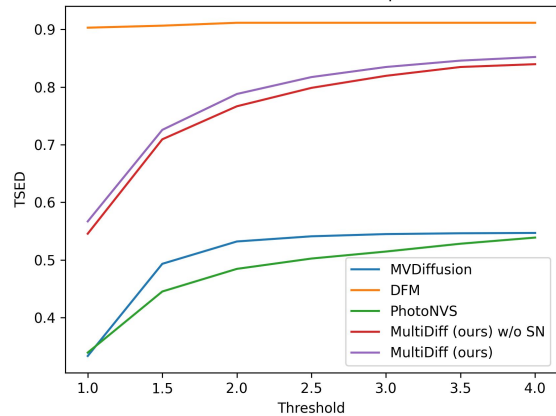

TSED@2px on ScanNet at 128px resolution

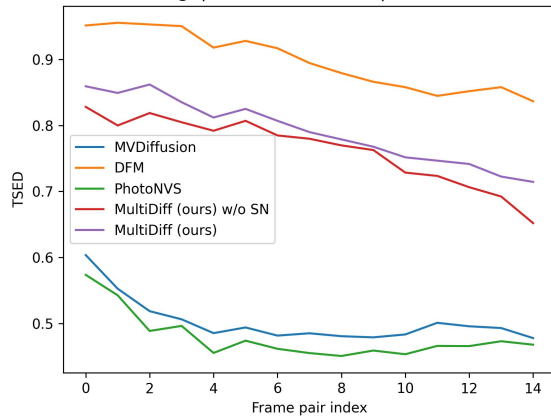

Supplement: Supplementary file 1 [file TSED_curves.pdf]
