# Supplementary material for: MultiDiff: Consistent Novel View Synthesis from a Single Image
Source: arXiv:2406.18524 source file (2024-06-26)

Sampled views

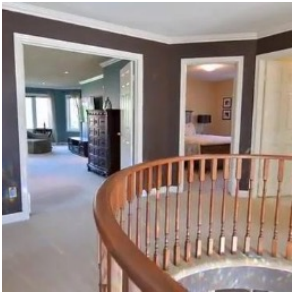

Reference image

Sample 1

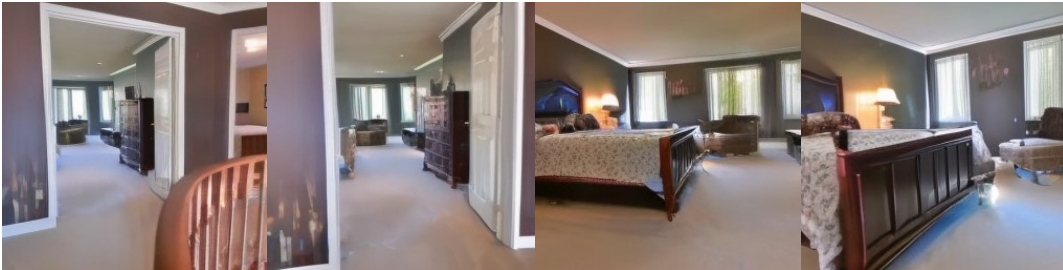

Sample 2

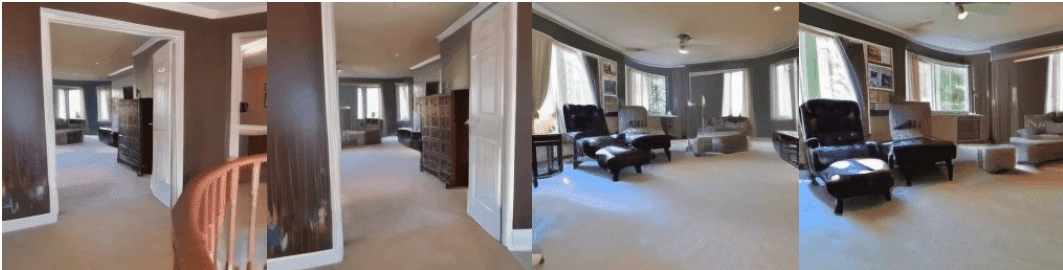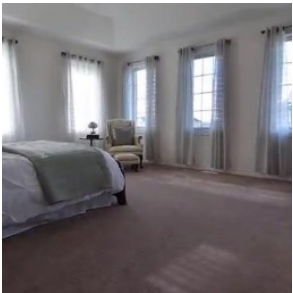

Reference image

Sample 1

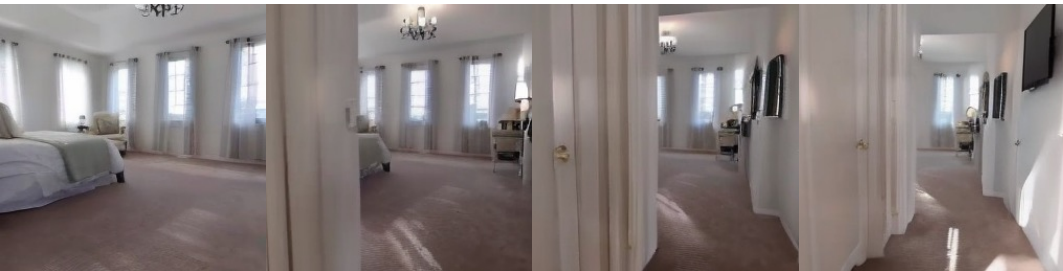

Sample 2

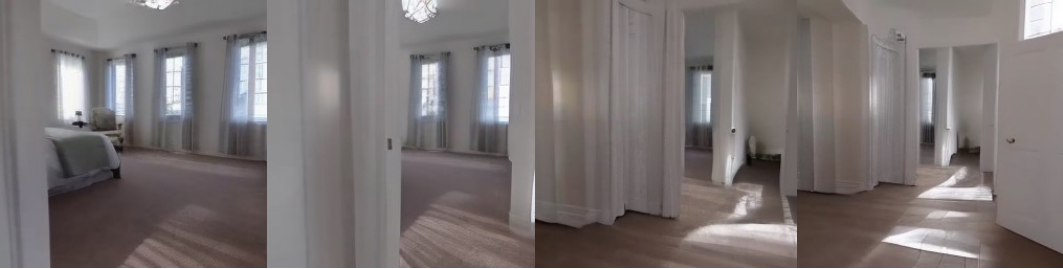



Reference

Sampled views →

DFM

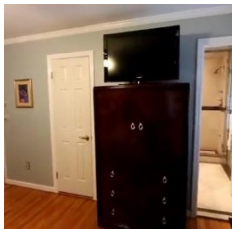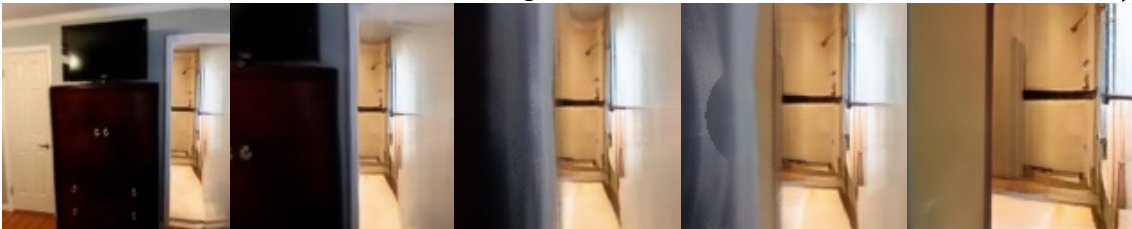

PhotoNVS

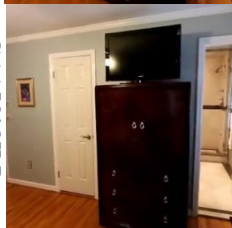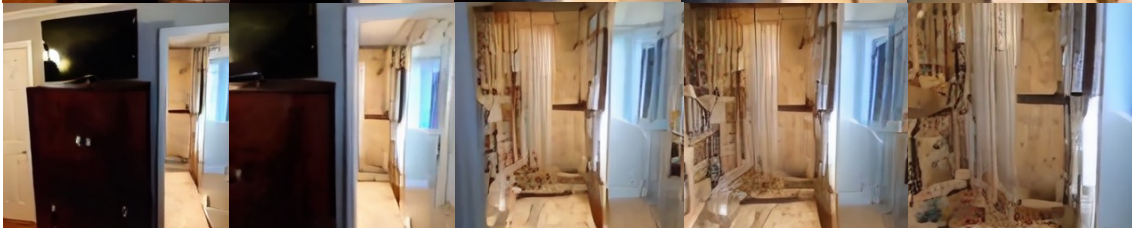

Ours

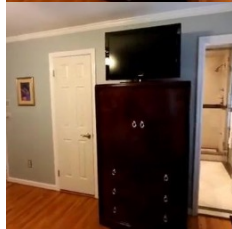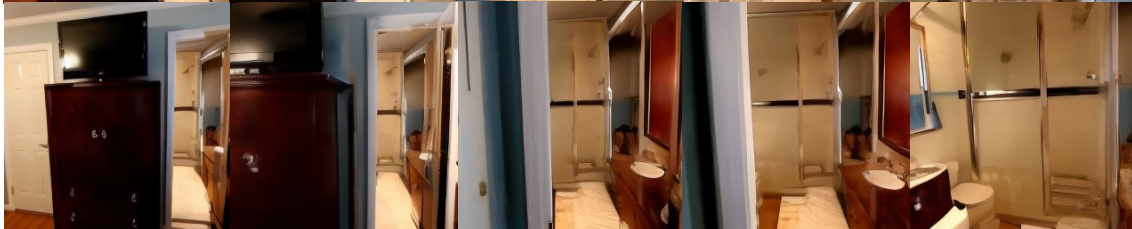

DFM

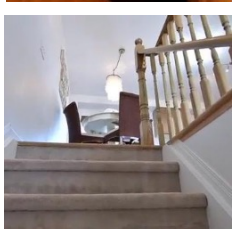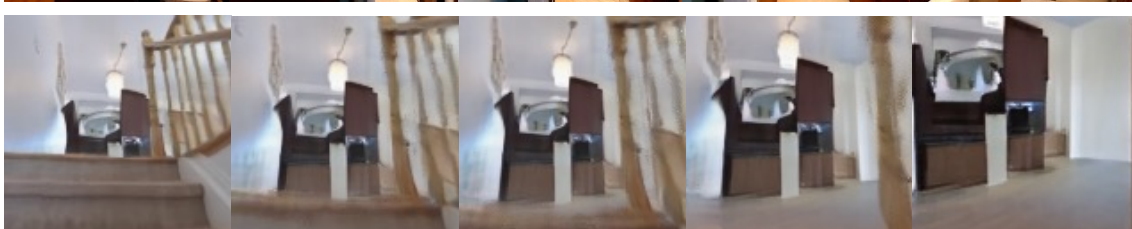

PhotoNVS

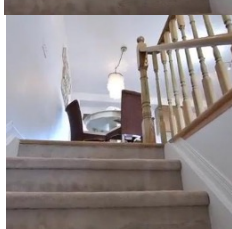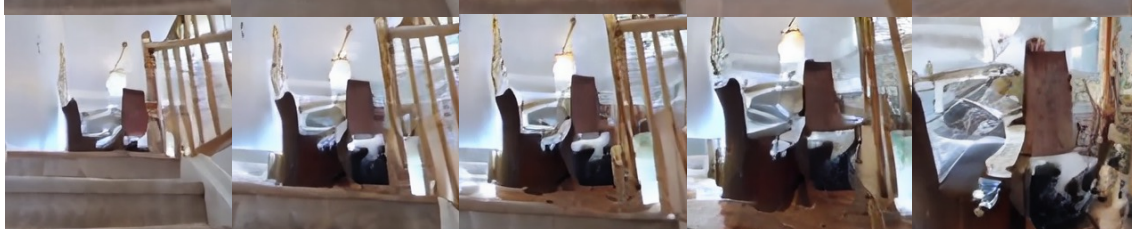

Ours

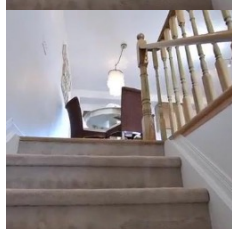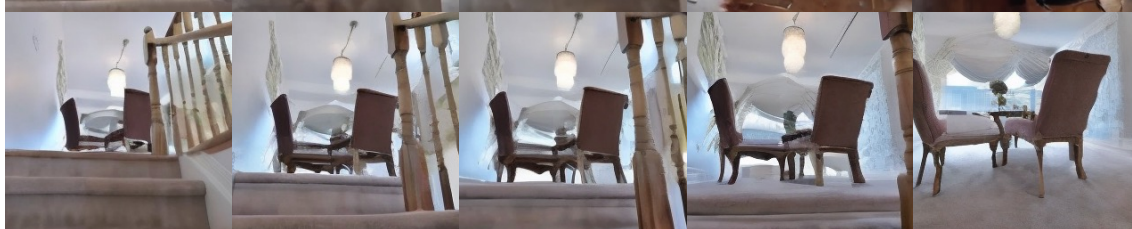

DFM

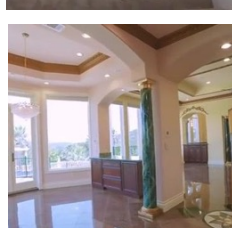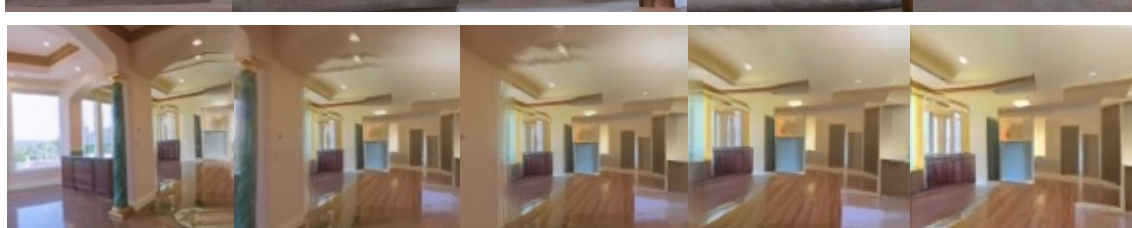

PhotoNVS

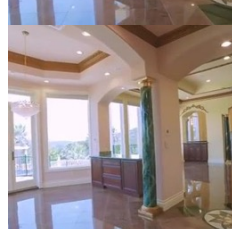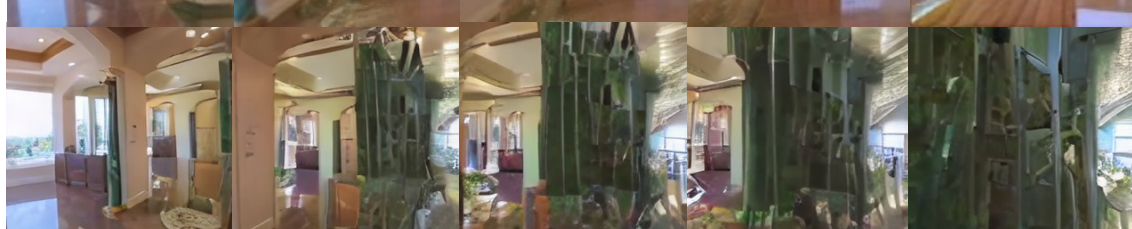

Ours

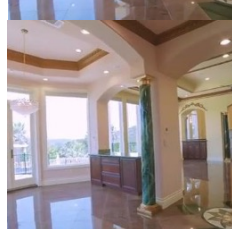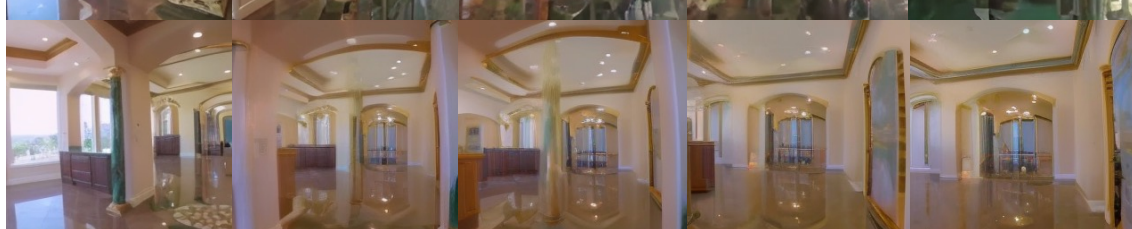



Reference

Sampled views

Ours

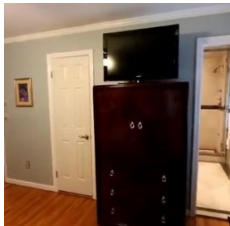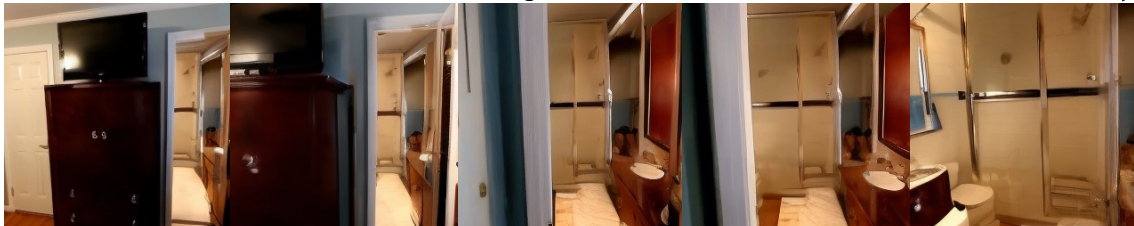

PhotoNVS

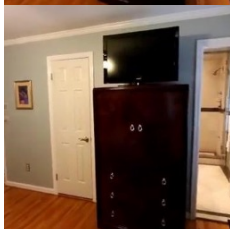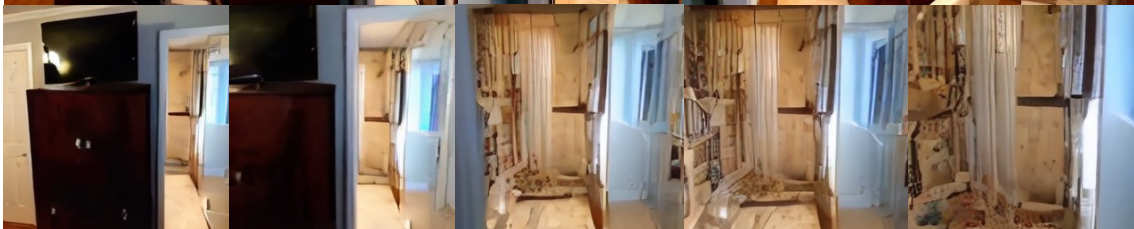

DFM

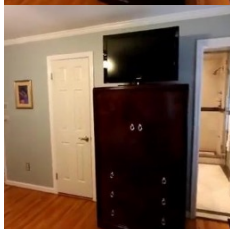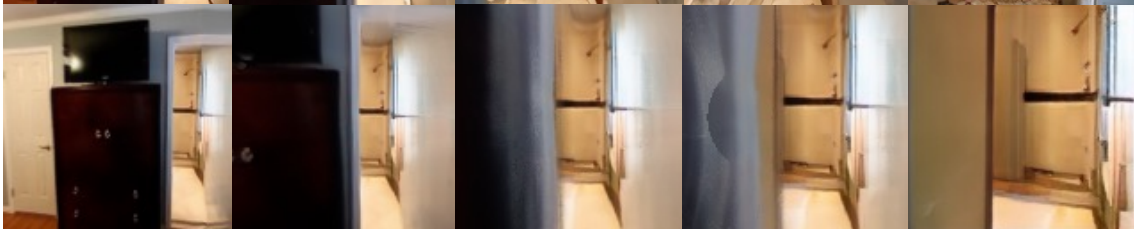

Ours

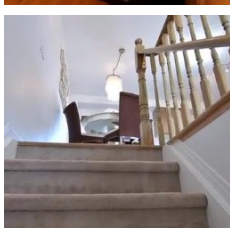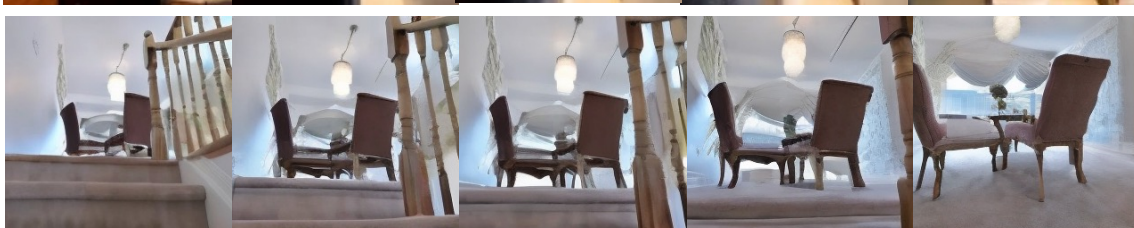

PhotoNVS

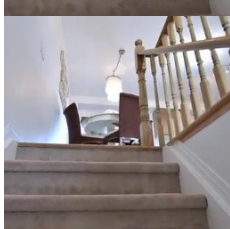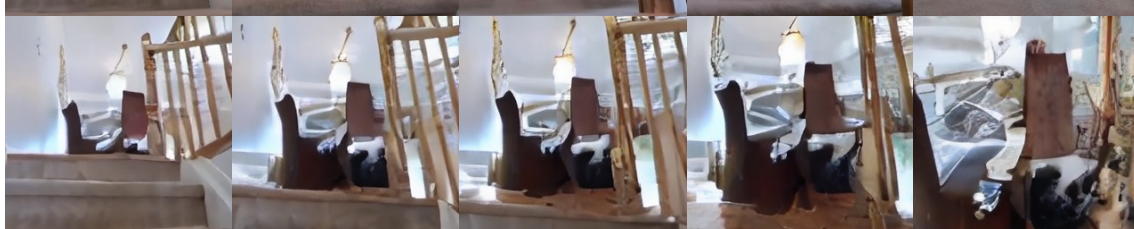

DFM

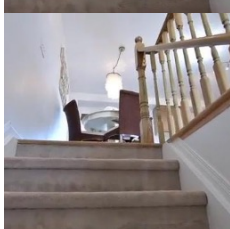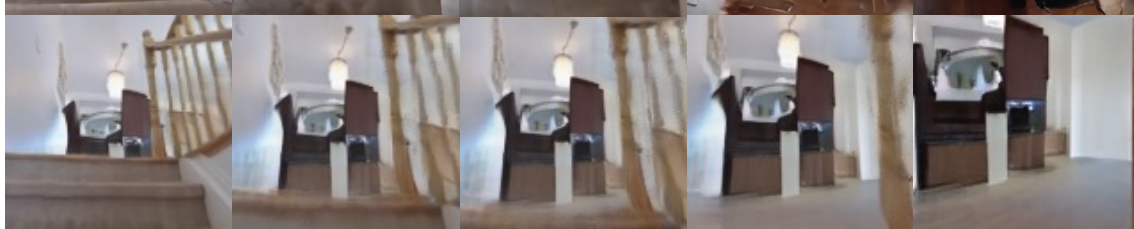

Ours

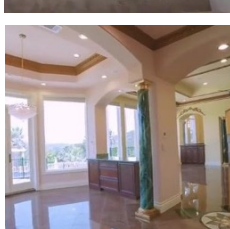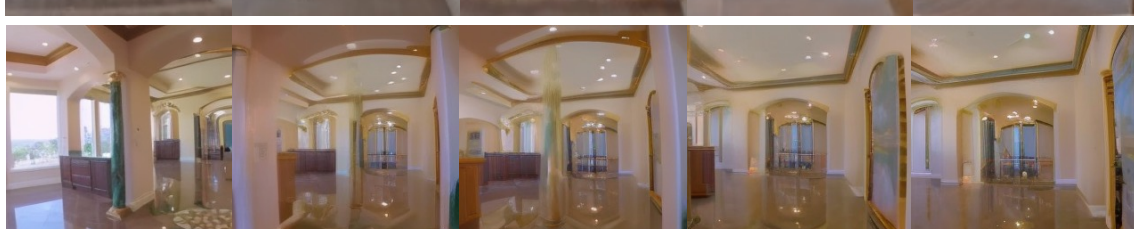

PhotoNVS

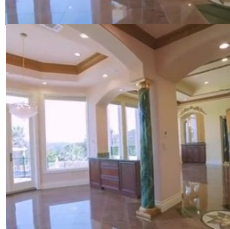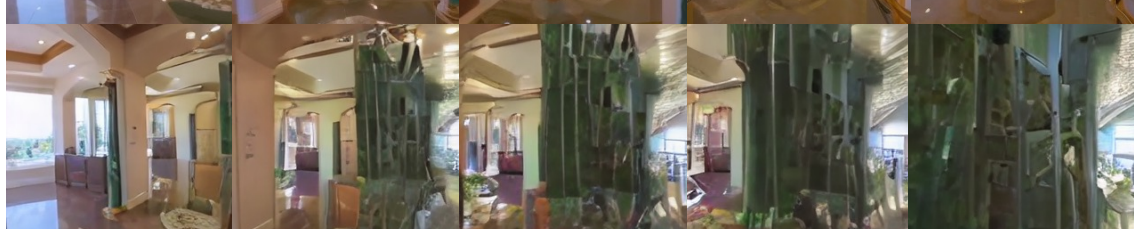

DFM

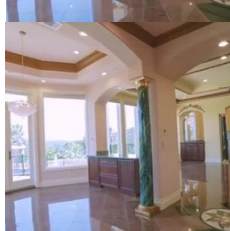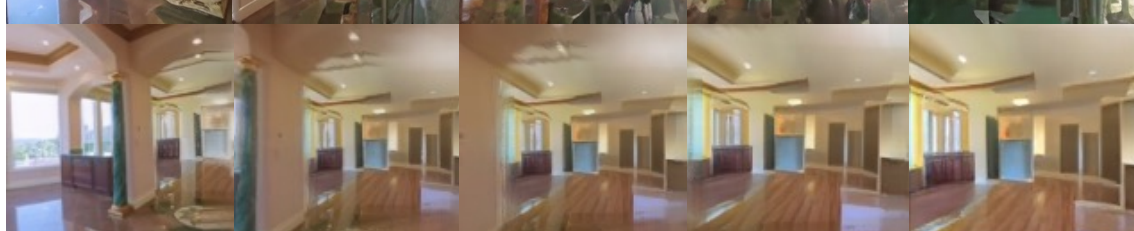



Reference image

Sampled views

Ours

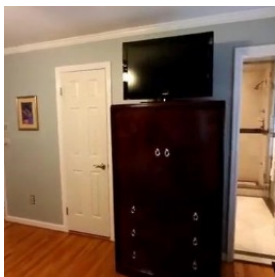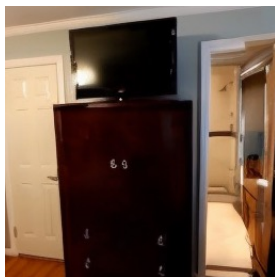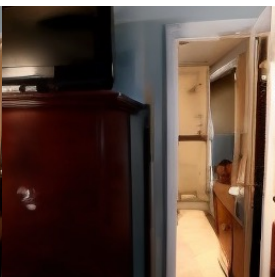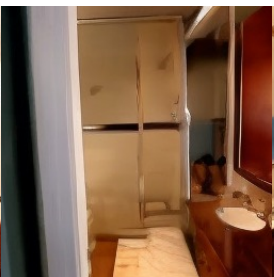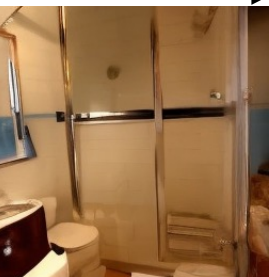

PhotoNVS

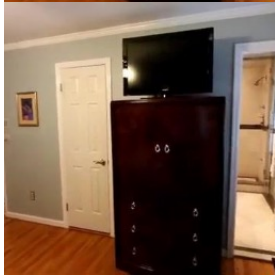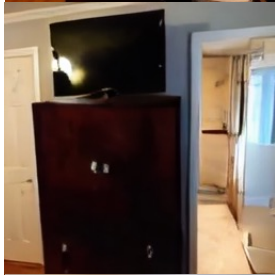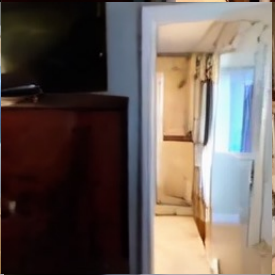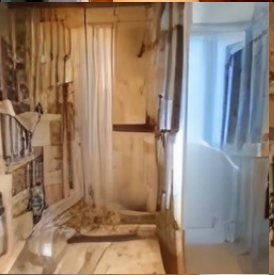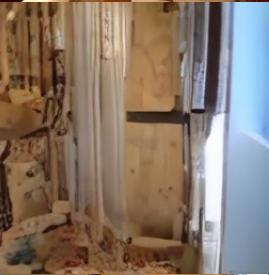

DFM

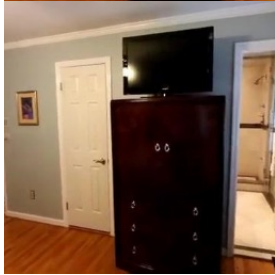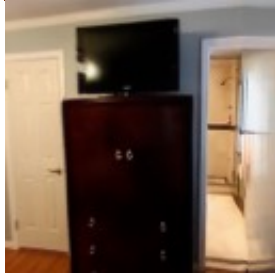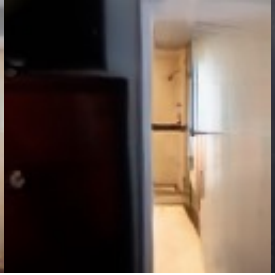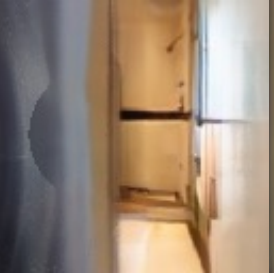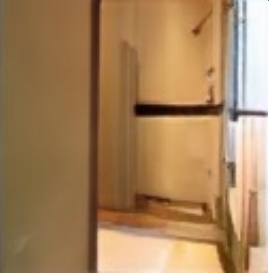

Ours

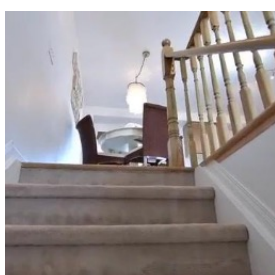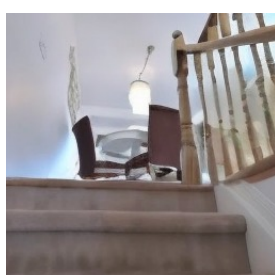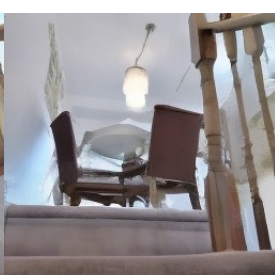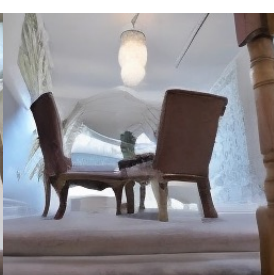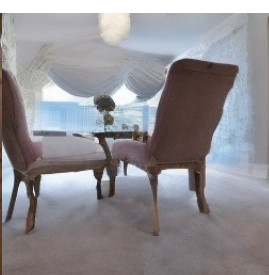

PhotoNVS

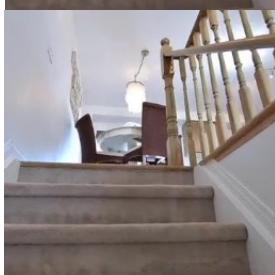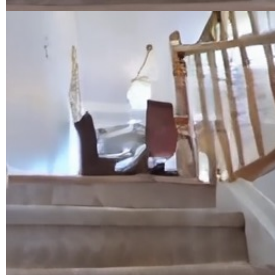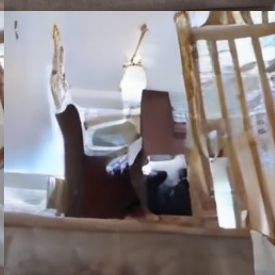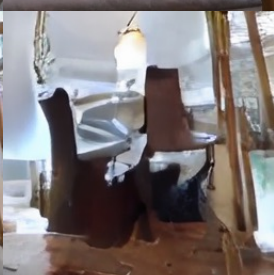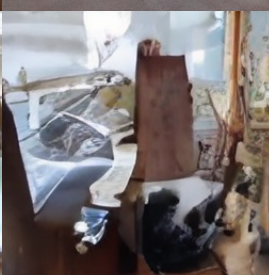

DFM

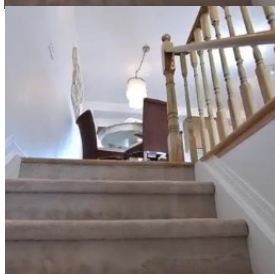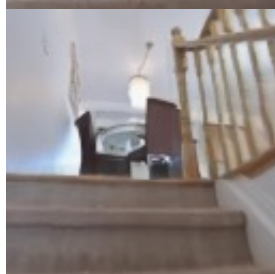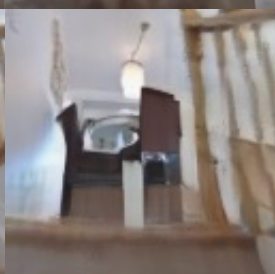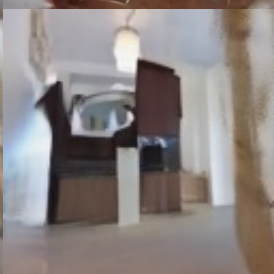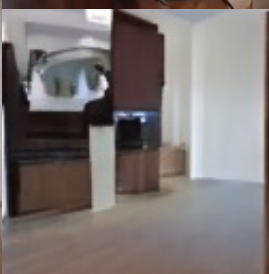

Ours

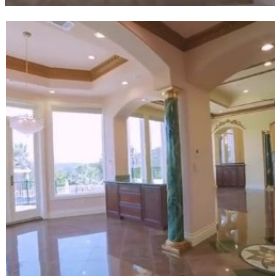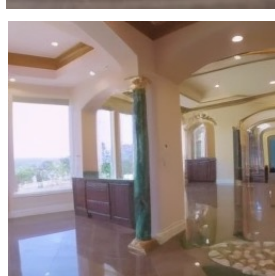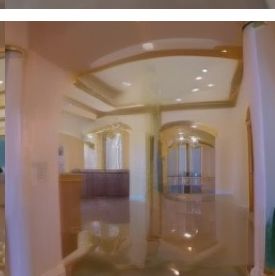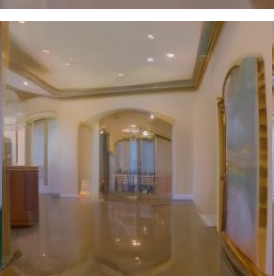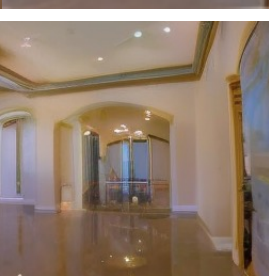

PhotoNVS

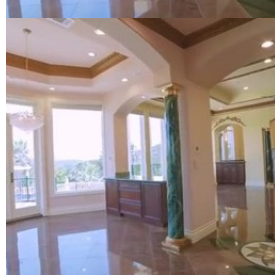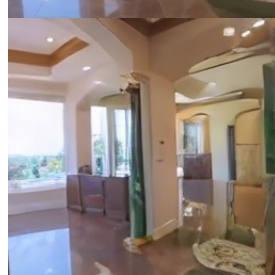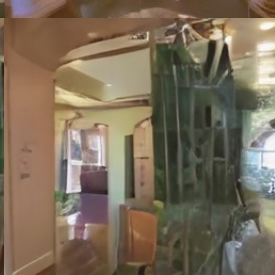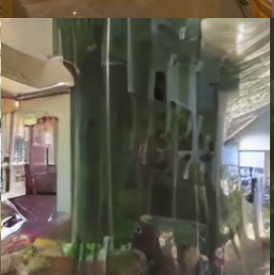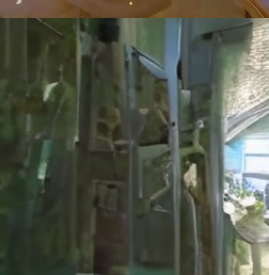

DFM

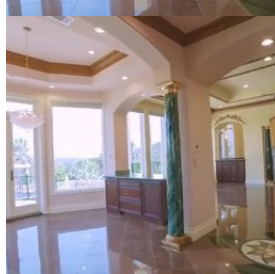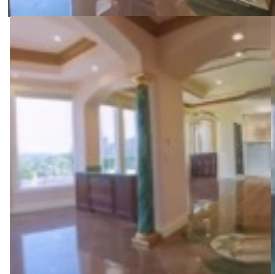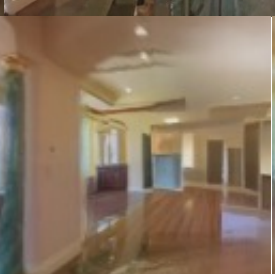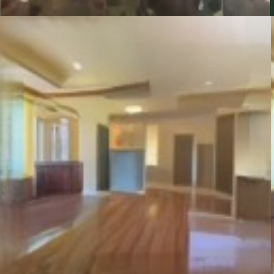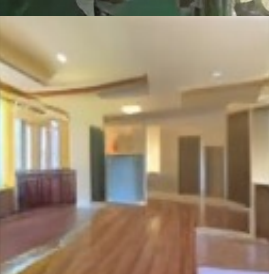



Reference image

Sampled views

Ours

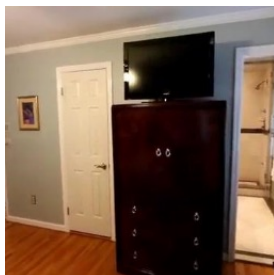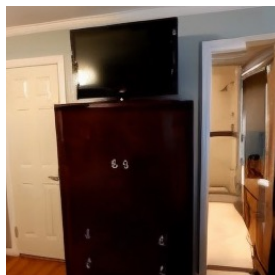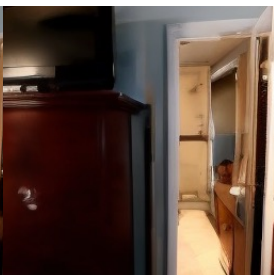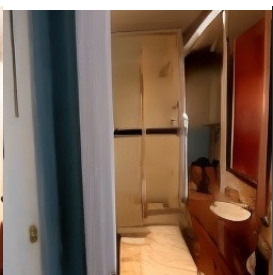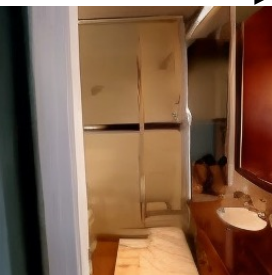

PhotoNVS

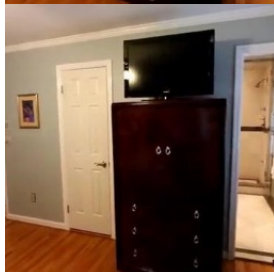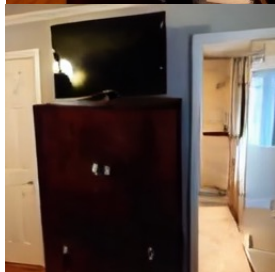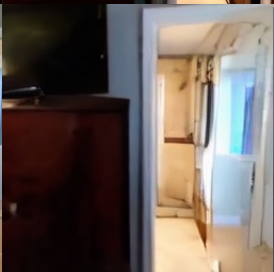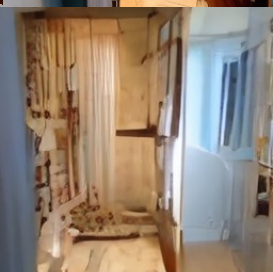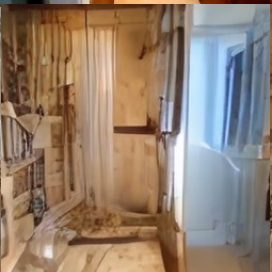

DFM

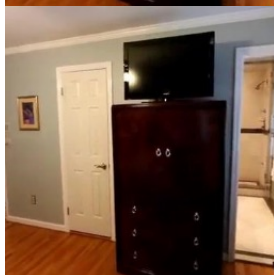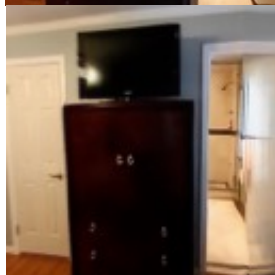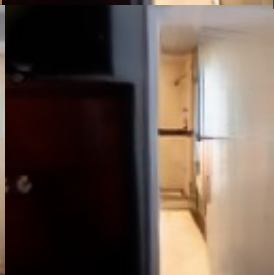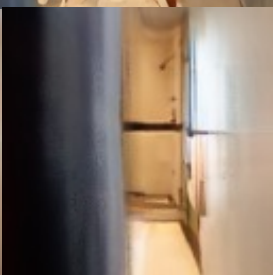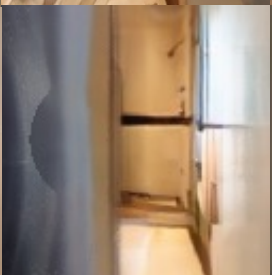

Ours

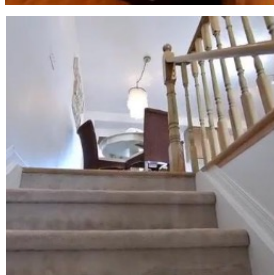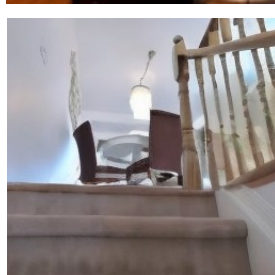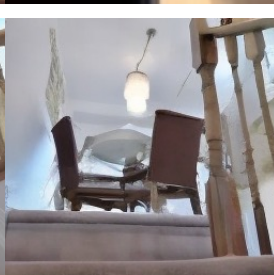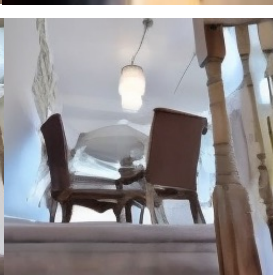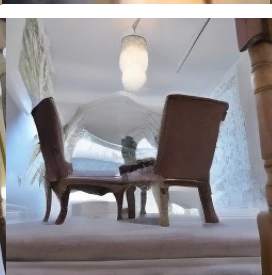

PhotoNVS

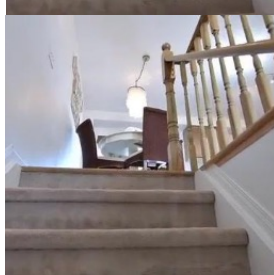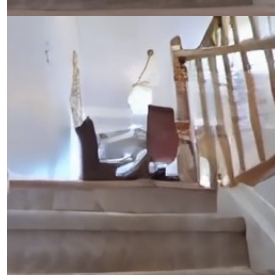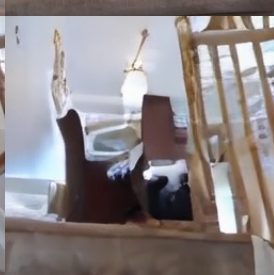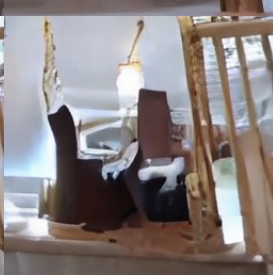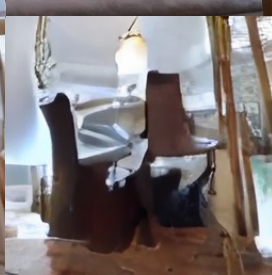

DFM

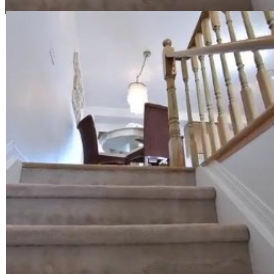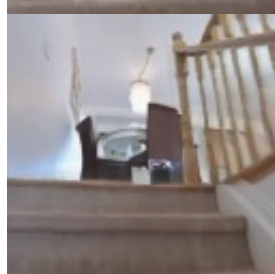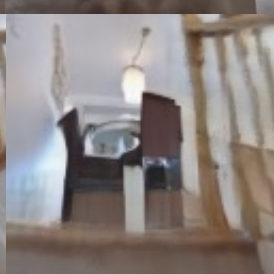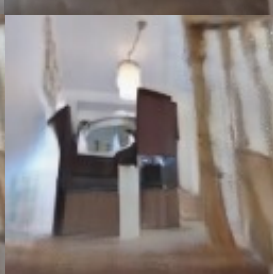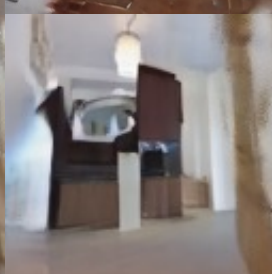

Ours

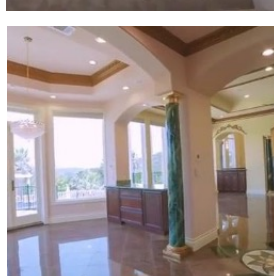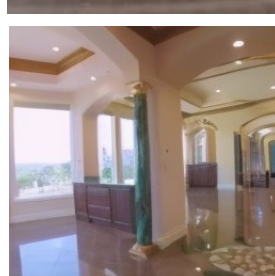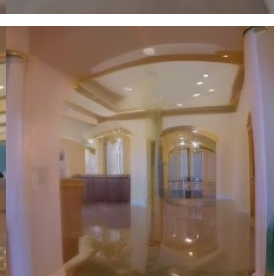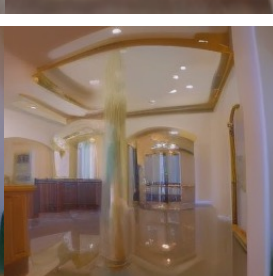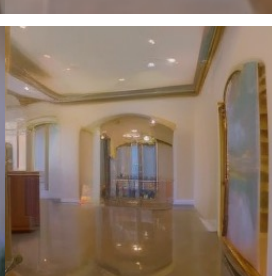

PhotoNVS

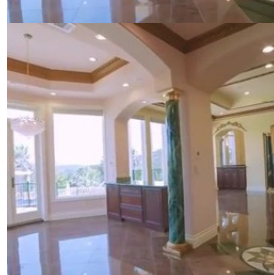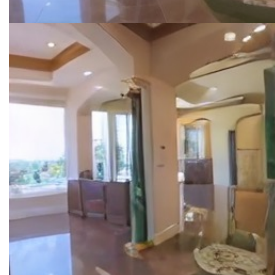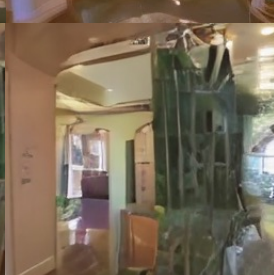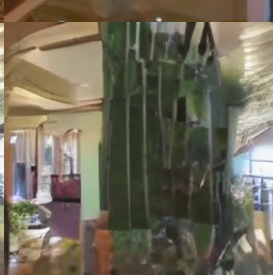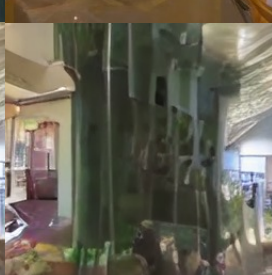

DFM

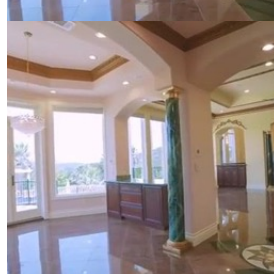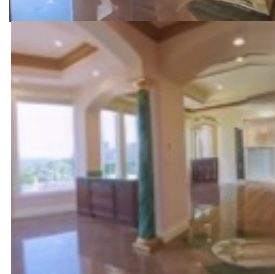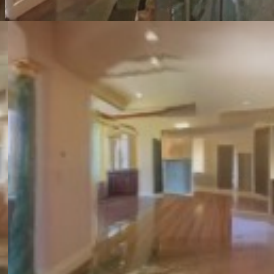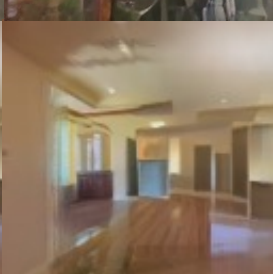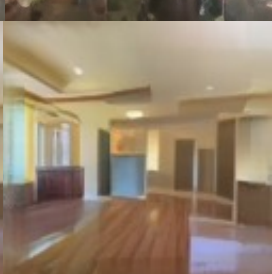



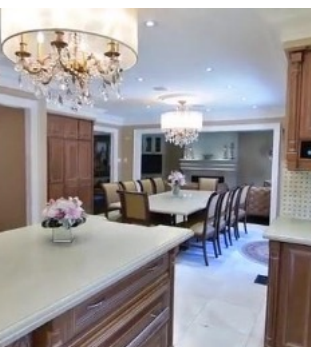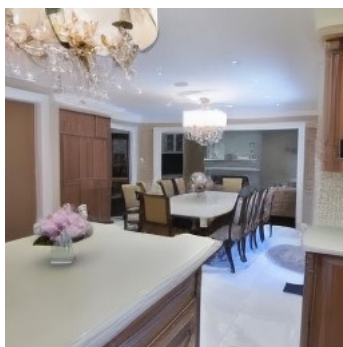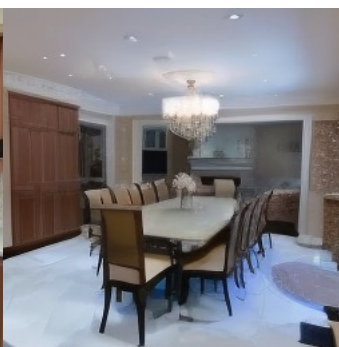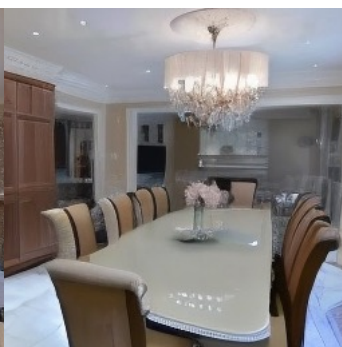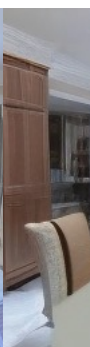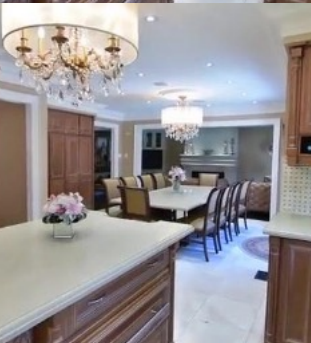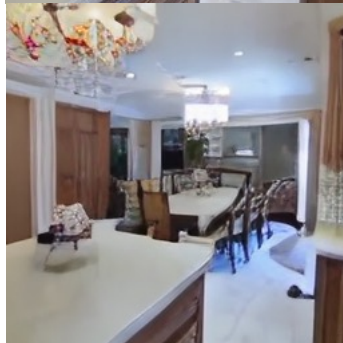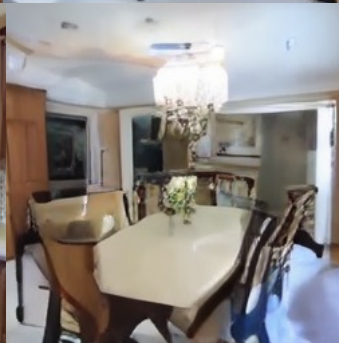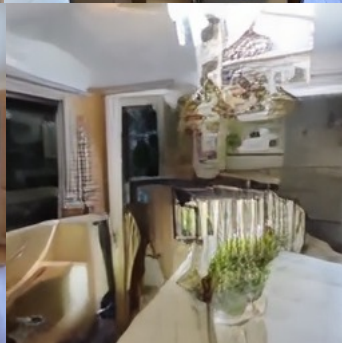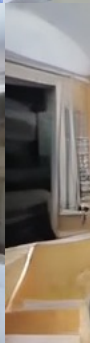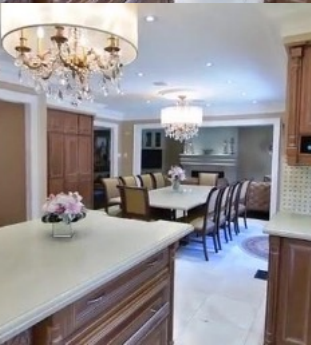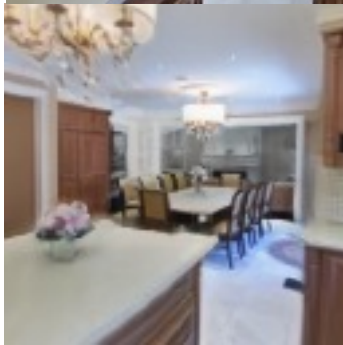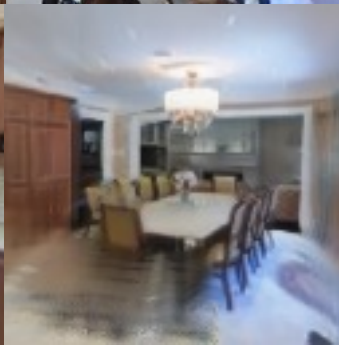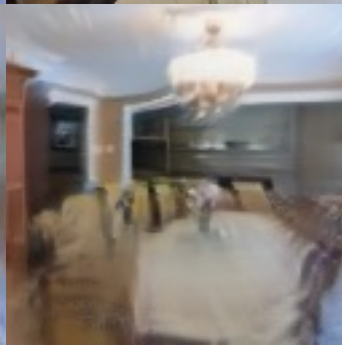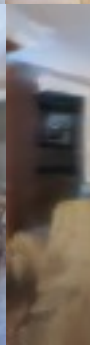



Reference

Sampled views

Ours

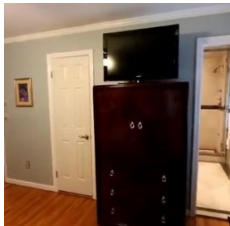

PhotoNVS

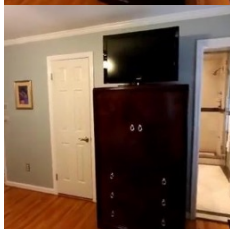

DFM

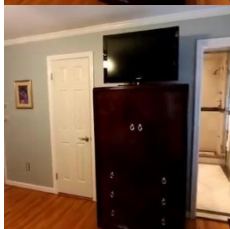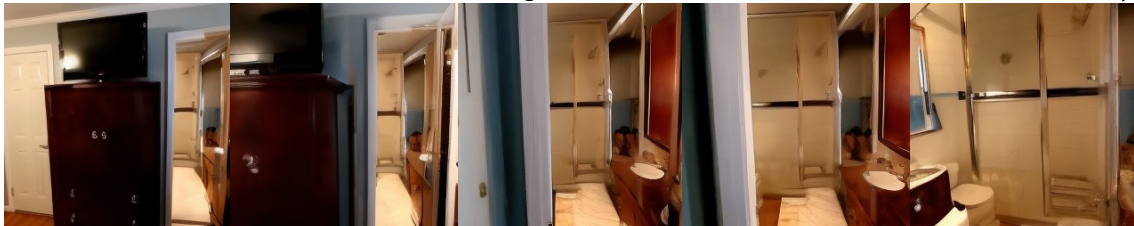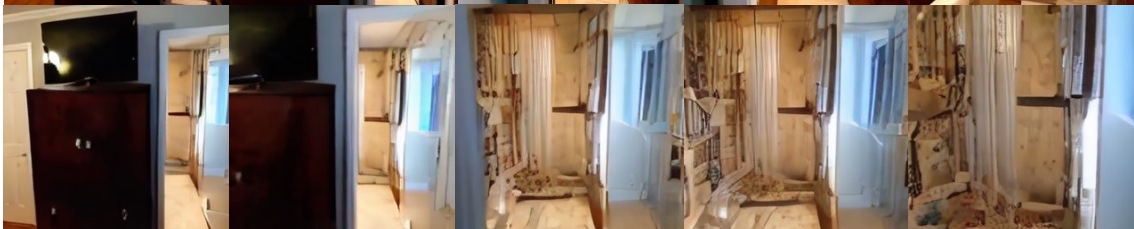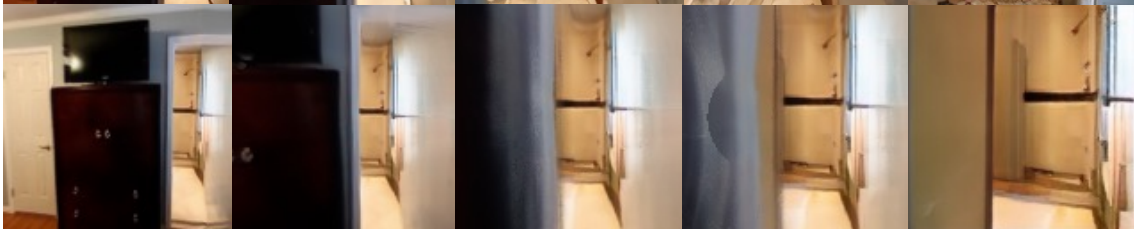

Ours

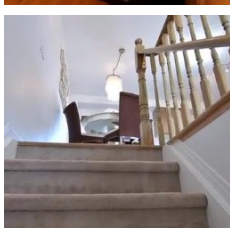

PhotoNVS

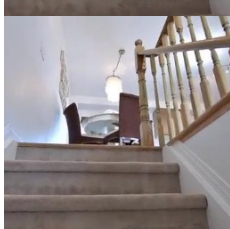

DFM

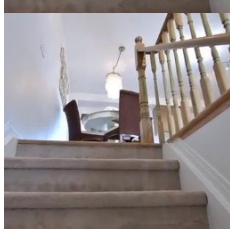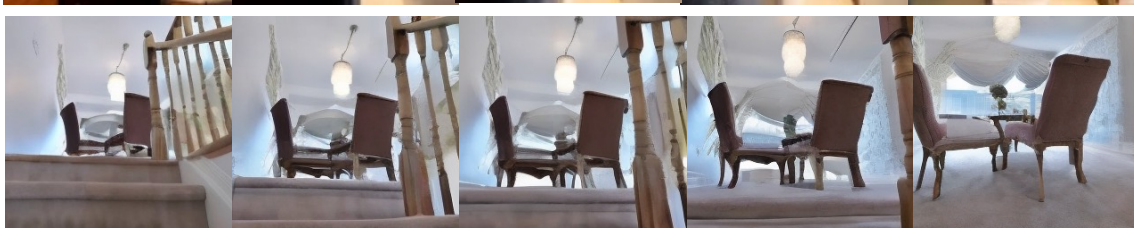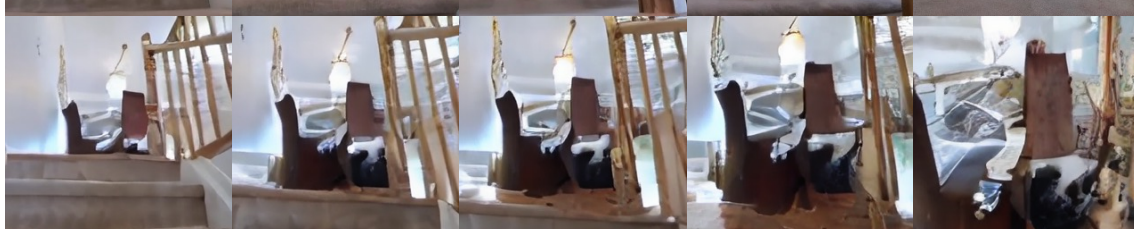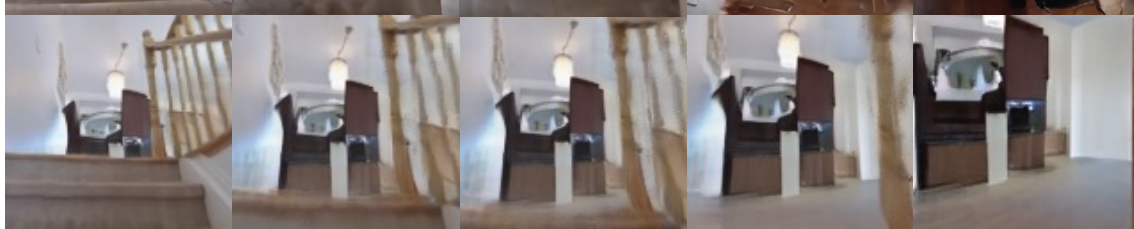

Ours

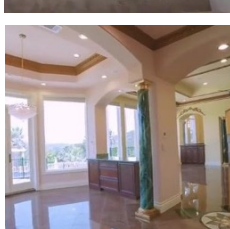

PhotoNVS

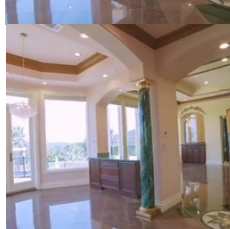

DFM

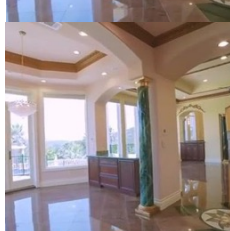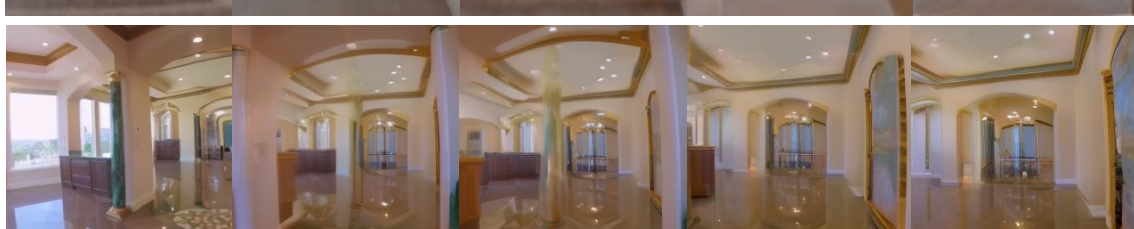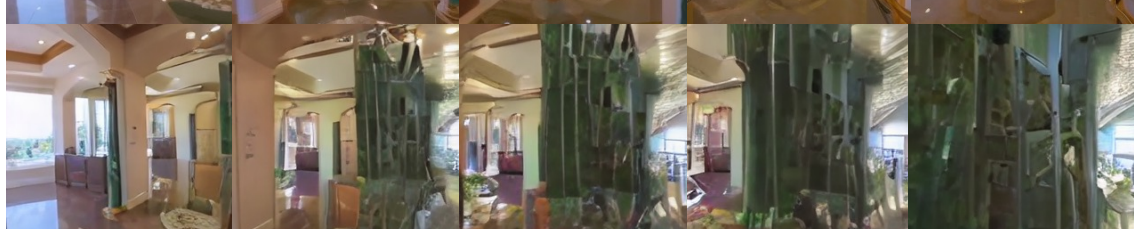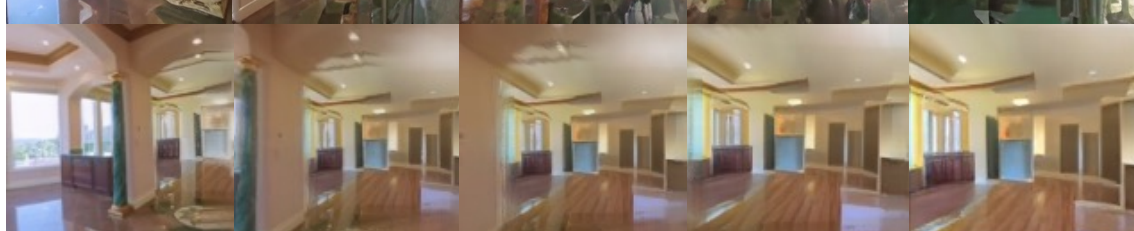

Supplement: Supplementary file 2 [file MultiDiff_suppl_re10k.pdf]
